# Supplementary material for: Elastometry of Deflated Capsules: Elastic Moduli from Shape and Wrinkle Analysis
Source: arXiv:1309.3124 source file (2013-09-12)
Supplement: Supplementary file 1 [file supplement_reduced.pdf]

Supplementary Information for

# Elastometry of Deflated Capsules: Elastic Moduli from Shape and Wrinkle Analysis

S. Knoche, D. Vella, E. Aumaitre, P. Degen,
H. Rehage, P. Cicuta and J. Kierfeld

22nd August 2013

## Contents

**1 Contour Analysis of Images** **2**

**2 Results for OTS and HFBII capsules** **5**

# 1 Contour Analysis of Images

Consider an image of a pendant capsule which has to be compared to a theoretical contour given by a parametrisation $r(s_0)$, $z(s_0)$ with $s_0 \in [0, L_0]$. The length unit of the theoretical contour is chosen as the capsule diameter $a$ at its upper rim, which coincides with the inner diameter of the capillary.

**Extracting Sampling Points.** The steps to find sampling points on the contour in an image are visualized in Fig. 1 and can be described as follows:

1. The images are imported as png files into Mathematica and converted into a matrix of greyscale values, which range from 0 (dark) to 1 (bright).
2. An edge detection algorithm (Canny's method, which is implemented in Mathematica) is used to find edges in the image.
3. The position of the end of the capillary is found by searching a horizontal jump in the upper part of the outermost edge (horizontal blue line).
4. All outermost points are detected. At the capillary (blue), they are used to determine the length scale of the image: The outer capillary diameter $b^{(px)}$ is measured in pixels. Its real dimensions (in mm) are known. At the capsule, the points (yellow) capture the contour.
5. Sampling points (red) are distributed equidistantly (each 5 pixels) along the contour.

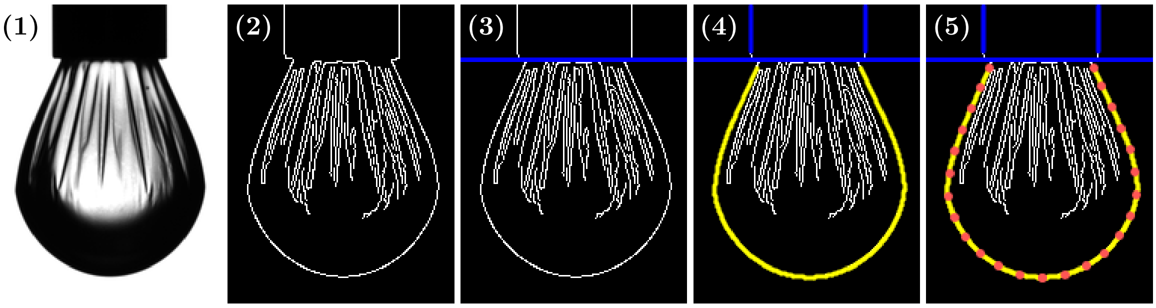


Figure 1: The five stages of the contour detection using the example of an OTS capsule, as described in the enumeration in the text.

**Deviation from Axisymmetry.** In some cases, the capsule in the image is inclined, because of a maladjusted camera or tilted table. Thus it does not seem to be axisymmetric with respect to the vertical axis. To compensate for this, the image has to be rotated by a certain angle, which is determined by minimizing the deviation from axisymmetry defined as follows (see Fig. 2):

For each pixel row, the difference between the center $(x_L + x_R)/2$ in this row and the $x$-coordinate $x_{cm}$ of the center of mass of all contour points (yellow) is squared and added to the error,

$$\delta_{axi} = \frac{1}{n} \sum_{\text{all rows}} \left( x_{cm} - \frac{x_L + x_R}{2} \right)^2 . \tag{1}$$

If necessary, each image is rotated by the angle that minimizes this error.

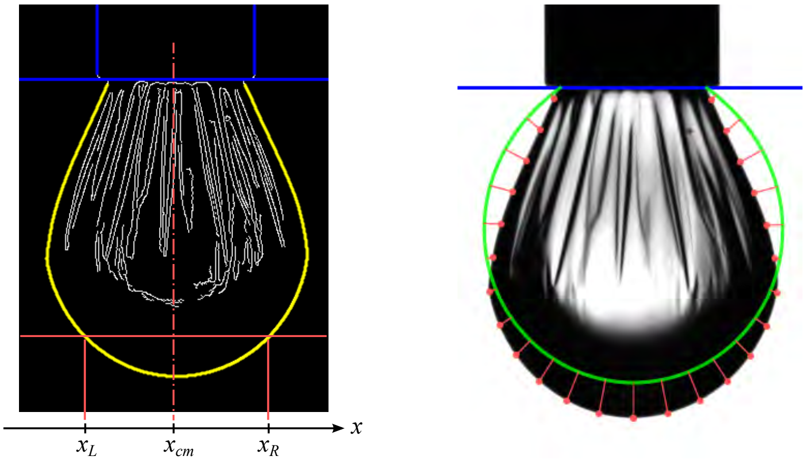


Figure 2: Left: Principle for calculating the deviation from perfect axisymmetry. Right: Measure of deviation between the theoretical contour (green line) and the sampling points (red). The shortest connections of the sampling points to the theory line (red lines) are squared and summed up.

**Measure of Deviation between Theory and Image.** All computed contours are nondimensionalised. Specifically, the length unit is given as the diameter of the capsule's upper rim. In order to compare a computed contour to the sampling points, we have to determine a conversion factor $a^{(\mathrm{px})}$ measuring the diameter in pixels. The contour measured in pixels is then given by

$$\begin{pmatrix} r^{(\mathrm{px})} \\ z^{(\mathrm{px})} \end{pmatrix} = a^{(\mathrm{px})} \begin{pmatrix} r(s_0) \\ z(s_0) \end{pmatrix} . \tag{2}$$

Now we can define a measure of how much a given theoretical curve $r^{(\mathrm{px})}$, $z^{(\mathrm{px})}$ deviates from the set of sampling points $\boldsymbol{x}_i^{(\mathrm{px})}$. In a geometrical language, the procedure can be described as follows.

- Lay the theoretical contour over the image, aligning its upper rim with the end of the capillary and the origin of the $r$-axis with the center of mass of the sampling points.
- Sum up the squares of the distances $d_i$ between $\boldsymbol{x}_i^{(\mathrm{px})}$ and the theoretical contour (see Fig. 2) and calculate the *root mean square deviation* (RMS deviation) over all $n$ sampling points:

$$\mathrm{RMS} \equiv \sqrt{\frac{1}{n}\sum_{i=1}^{n} d_i^2}. \tag{3}$$

**Scaling Factors.** Unfortunately, $a^{(\mathrm{px})}$ cannot be measured directly from the images because the point of attachment between capillary and capsule frequently accumulates dirt like patches of the polymerized material. So we decided to determine $a^{(\mathrm{px})}$ indirectly with the Laplace Young fits: We adjust $a^{(\mathrm{px})}$ so that the Laplace-Young fits have the lowest remaining RMS deviation, i.e. we use the scaling factor as an additional fit parameter. The mean value $\left\langle a^{(\mathrm{px})} \right\rangle$ of all Laplace-Young fits is then kept for all following fits of the elastic shape equations.

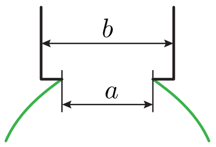


Figure 3: Capillary measures

In addition to the conversion factor $a^{(\mathrm{px})}$ between theory length unit and pixels, we need to know the diameter in real length units, e.g. in millimeters. Since the outer diameter $b^{(\mathrm{mm})}$ (see Fig. 3) of the capillary is specified by the manufacturer, we can calculate the inner diameter as

$$a^{(\mathrm{mm})} = \left\langle a^{(\mathrm{px})}/b^{(\mathrm{px})} \right\rangle \cdot b^{(\mathrm{mm})}, \tag{4}$$

where the average $\langle\cdot\rangle$ is taken over all pictures that are used for the Laplace-Young fits.

**Estimating errors coming from the contour detection.** Our contour detection has a resolution of $\pm 1$ pixel. The worst case would be that the points are shifted systematically. In order to estimate how strong this worst-case error in the contour detection influences the fit results, we repeat the fits with misplaced contour points in the image of the deformed capsule. The misplacements are done in four different modes:

- Shift all contour points by 1 pixel outward.
- Shift all contour points by 1 pixel inward.
- Shift the points on the side inward, and the points at the bottom downward (so that the capsule appears more slender).
- Shift the points on the side outward, and the points at the bottom upward (so that the capsule appears more chubby).

The error bars for the points in the $V$-$K_{2D}$- and $V$-$\nu_{2D}$-diagrams (Fig. 4 in the main text) are generated by taking the maximum deviation from the original results. If the maximum deviation is still smaller than the grid spacing on the $K_{2D}$ or $\nu_{2D}$ axes, we take the grid spacing as the smallest possible error bar. Hence, they are worst-case-estimates. Typically, the inward/outward modes produce the largest deviations in $V/V_0$, whereas the slender/chubby modes produce the largest errors in the elastic constants.

We expect the modes described above to reveal the worst case systematic errors of the method. Since they describe a possible systematic mistake of the camera, for example caused by lighting effects, we expect that all images are affected by the same mode. It follows that each point in the diagrams (Fig. 4 in the main text) has to be shifted in the same direction if they are corrected. Thus, the positions of the points relative to each other are mainly conserved. This ensures that the trends observed in the diagrams are well resolved; only the overall scale of the plot may vary within the error bars.

Another systematic error comes from the fact that the pseudo-surface deviates from the detected outermost contour about 1 wrinkle amplitude. Especially for OTS capsules, where the wrinkle amplitude grows larger than 1 pixel during deflation, it has to be checked that this error is smaller than the observed drift of the compression modulus.

For given wavelength $\Lambda$, the $s_0$-dependent wrinkle amplitude is determined by the consideration that a circumferential fibre of real length $W(s_0) = 2\pi r_0 \lambda_\phi$ must be deposited on the perimeter $U(s_0) = 2\pi r_0 \bar{\lambda}_\phi$ of the pseudo-surface. In the wrinkling region where $\bar{\lambda}_\phi < \lambda_\phi$, there is an excess length $W(s_0) - U(s_0) > 0$ which has to lie in the wrinkles. For sinusoidal wrinkles with small amplitude $A$, the excess length is given as

$$W - U = \int_0^U \frac{1}{2} \left( \frac{d}{dx} (A \sin(2\pi x/\Lambda) \right)^2 dx \tag{5}$$

$$= \int_0^U \frac{2\pi^2 A^2}{\Lambda^2} \cos^2(2\pi x/\Lambda)\, dx = \frac{\pi^2 A^2 U}{\Lambda^2}, \tag{6}$$

where the integration was performed with the assumption that $U$ is a multiple of a full period of the $\cos^2$ term. This gives the relation

$$2\pi r_0 (\lambda_\phi - \bar{\lambda}_\phi) = \frac{\pi^2 A^2 2\pi r_0 \bar{\lambda}_\phi}{\Lambda^2} \tag{7}$$

so that the amplitude reads

$$A(s_0) = \frac{\Lambda}{\pi} \sqrt{\left( \frac{\lambda_\phi(s_0)}{\bar{\lambda}_\phi(s_0)} - 1 \right)}. \tag{8}$$

Now, instead of measuring the RMS deviation between midsurface $(r(s_0), z(s_0))$ and sampling points, we measure it between the outermost surface $(r(s_0) + A(s_0), z(s_0))$ and sampling points.

Surprisingly, the influence on the resulting fit parameters is small compared to the four misplacement modes discussed above, although the maximum amplitude is 5 pixels. Only the capsule volume is affected significantly, so that the points in the $V$-$K_{2D}$-diagram (Fig. 4 in the main text) would be shifted to the left and would change the slope of the linear fit a bit. For clarity, this error mode is not presented in detail in the main text since it is less significant than the modes mentioned before.

# 2 Results for OTS and HFBII capsules

**Step 1: Laplace-Young fits and conversion factors.** In both OTS and HFBII measurements, four images of the undeformed capsule were fitted with the Laplace-Young equation with the interfacial tension $\gamma$, internal pressure $p_0$ and scaling factor $a^{(px)}$ as fit parameters. The averaged surface tensions and conversion factors are listed in the table below.

| | $\gamma$ | mm $\leftrightarrow$ px | theor. length unit $\leftrightarrow$ px |
|---|---|---|---|
| OTS | 11.2 mN/m | 1 mm$\hat{=}$135 px | 1$\hat{=}$194 px |
| HFBII | 49.8 mN/m | 1 mm$\hat{=}$146 px | 1$\hat{=}$139 px |

Whereas the Laplace-Young fits for HFBII match the detected contour nearly perfectly, small systematic deviations ($\pm 1$ px) can be observed for the Laplace-Young fits to the initial OTS capsule. These deviations can be explained by the polymerization process and might affect the results of the following elastic fits, especially for small deformation.

**Step 2: Shape Analysis.** In this section, we will discuss a representative set of plots (Fig. 4) of the fit results for OTS and HFBII capsules.

A visual check whether the fits have been successful can be done by plotting the fitted contour over the capsule image (upper left figure in each panel of Fig. 4). Evidently, the capsule shapes are reproduced very well. For the OTS capsule, even the boundary of the wrinkled region predicted by the theory (horizontal green lines) matches the experimental result; although the position of the horizontal green lines was *not* incorporated in the RMS deviation. The fact that they coincide with the experimental observations proves that the elastic model captures the wrinkling behavior accurately. For the hydrophobin capsule, the wrinkled region cannot be seen in the image, because the wrinkles have sub-pixel dimension. The visible folds are only secondary structures.

In order to check whether the RMS deviation minimum is found correctly, we present a plot of the RMS deviation distribution in the $(K_{2D}, \nu_{2D})$-plane (upper right figure in each panel of Fig. 4). The plots show that the minimum is nicely located inside the refined area of the parameter space. That was facilitated by choosing the area compression modulus $K_{2D}$ instead of the surface Young modulus $Y_{2D}$ on the horizontal axis. The reverse mapping $Y_{2D} = 2(1 - \nu_{2D})K_{2D}$ would stretch the circular minimum to a long and narrow ellipse, which would be harder to analyze with our rudimentary grid based minimization method.

Finally, the fit residual along the contour (bottom figure in each panel of Fig. 4) reveals whether there are systematic deviations between fitted contour and sampling points. In both cases, the systematic deviations are relatively small, though visible. For the OTS capsule, the largest deviations are at the right attachment point to the capillary, and other maxima at the point where the wrinkles end (around the 50$^{\text{th}}$ sampling point, see upper left figure). At this point, the capsule even seems to have a small kink, which cannot be reproduced by the model according to the continuity conditions of the slope angle. In case of the HFBII capsule, this effect is much smaller since the wrinkle amplitude is smaller. Consequently, the fit residual shows a less systematic behaviour.

**Step 3: Wrinkle analysis.** As described in the main text, the wrinkle analysis was only possible for the OTS capsule since the wrinkles on the HFBII capsule could not be resolved without microscopy. For OTS, the resulting bending stiffness is $E_B \approx (2.5 \pm 0.7) \cdot 10^{-14}$ Nm. We can use the well known

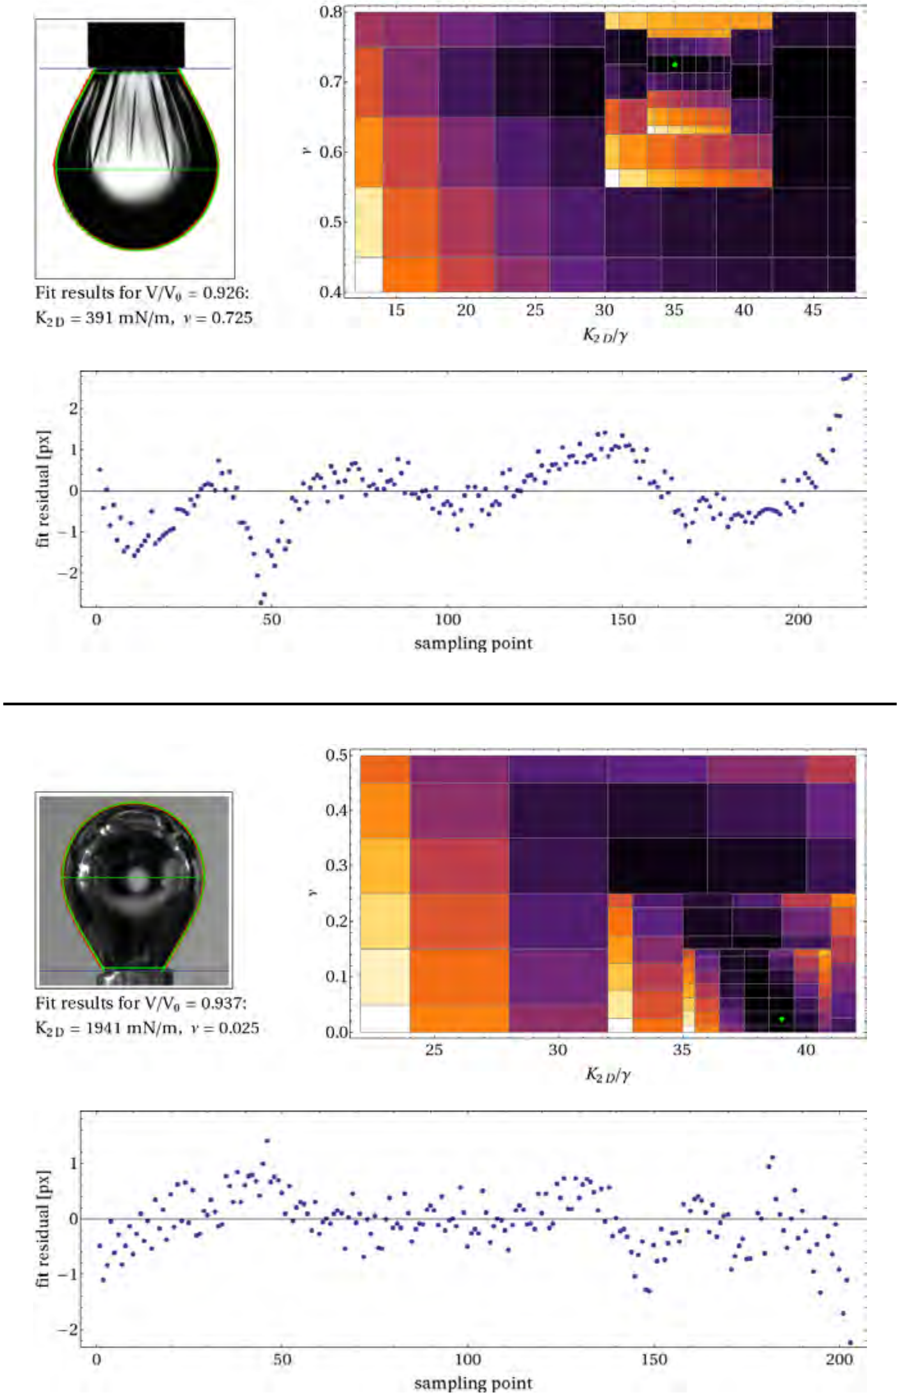


Figure 4: Fit result for a deflated OTS (upper panel) and hydrophobin (lower panel) capsule. On the upper left in each panel, the fitted contour (in green) is plotted over the image; the sampling points of the RMS deviation are shown in red in the background. The theory predicts the capsule to wrinkle between the horizontal green lines. On the upper right, the RMS deviation distribution in the $(K_{2D}, \nu_{2D})$-plane is plotted. Dark squares correspond to small deviation, light squares to large deviation. In the refinements, the colors are rescaled to cover the whole range. A green dot indicates the best result found. At the bottom, the fit residual along the contour (starting at the capillary, left side) is plotted to reveal possible systematic deviations.

relation from classical shell theory

$$E_B = \frac{Y_{2D} H_0^2}{12(1-\nu_{3D}^2)} \quad \Rightarrow \quad H_0 = \sqrt{12(1-\nu_{3D}^2)E_B/Y_{2D}} \tag{9}$$

to calculate the membrane thickness $H_0$ from the values for $E_B$, $Y_{2D}$ and $\nu$. This formula is valid for shells composed of a thin sheet of isotropic material, for which $\nu_{2D} = \nu_{3D}$. However, the Poisson ratio $\nu_{2D} \approx 0.6$ obtained for OTS capsules indicates that this cannot be the case, since $\nu_{3D} < 1/2$ for stability reasons. Hence the membrane thickness $H_0 \approx (0.77 \pm 0.07)\,\mu$m obtained from (9) should rather be considered as an *effective* thickness.

The results for the effective membrane thickness can be confirmed by raster electron microscopy measurements with another OTS capsule produced according to the same protocol (Fig. 5). During the preparation for the REM measurements, the membrane was dried and teared in consequence. At some gaps (numbered 1-4 in Fig. 5), values of $1.4\,\mu$m, $0.98\,\mu$m, $0.83\,\mu$m and $0.86\,\mu$m were obtained for the thickness. This agreement of the fitted and measured membrane thickness suggests that our method works accurately.

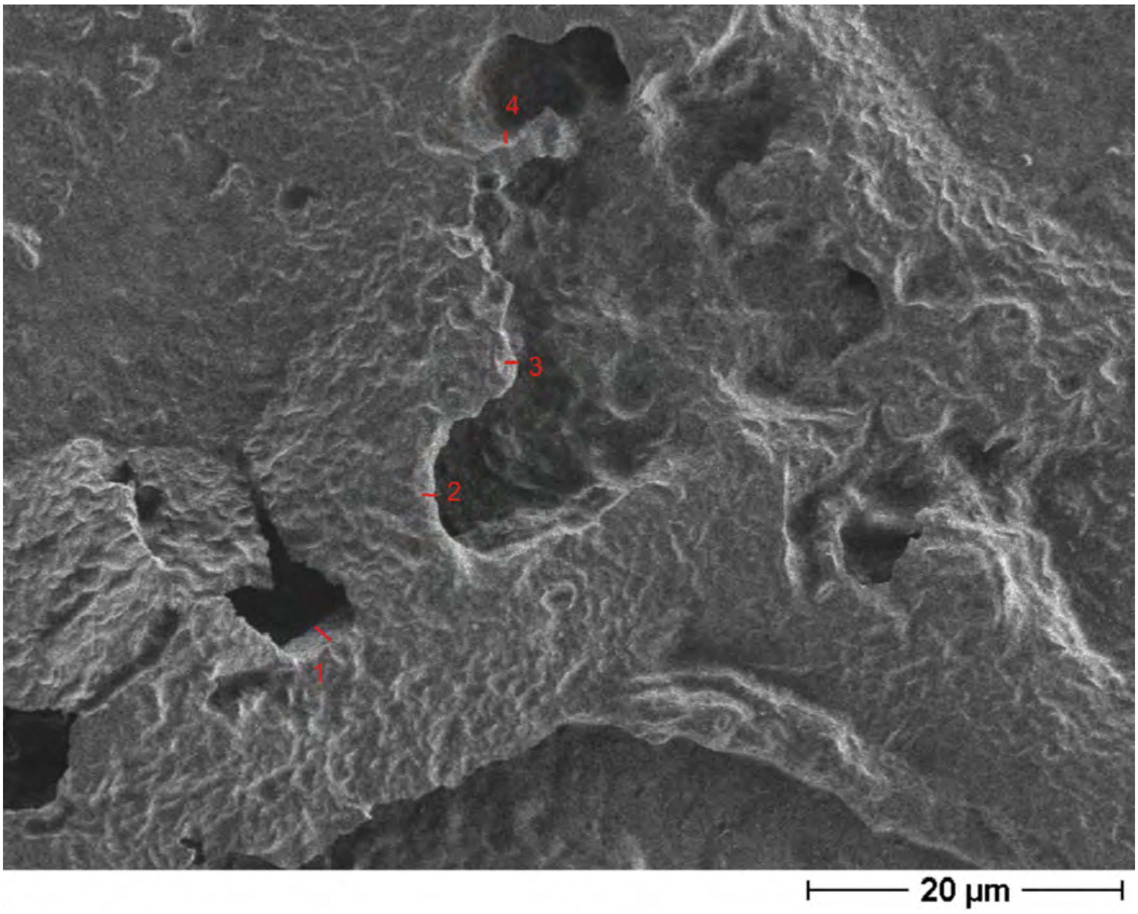


Figure 5: Raster electron microscopy image of a dried and torn OTS membrane. The numbered red lines indicate thickness measurements.
